# Supplementary material for: Unsupervised Denoising for Signal-Dependent and Row-Correlated Imaging Noise
Source: arXiv:2310.07887 source file (2025-04-07)
Supplement: Supplementary file 2 [file supp_figures.tex]

\newcommand\tabSz{
    \begin{table}[]
    \centering
    \label{tab:Sz}
    \begin{tabular}{c:c|c}
    $f_\nu(\cdot)$ & $\overline{\x} : \x\sim p_\theta(\x|\cdot)$ & RMSE \\ \hline
    $\z^1$ & $\z^1$ & 2.43 \\
    $\z^2$ & $\z^2$ & 2.45 \\
    $\z^1$ & $\z^2$ & 23.28 \\
    $\z^2$ & $\z^1$ & 23.31 \\
    \end{tabular}
    \end{table}
}

\newcommand\figSz{
\begin{figure}[h]
    \centering
    \includegraphics[width=\linewidth]{supp_figures/isszexz.pdf}
    \caption{Given a noisy image $\x$, we took two samples from the approximate posterior, $\z_1$ and $\z_2$.
    For each latent variable sample, we produced one estimate of the signal by passing it through the signal decoder $f_\nu$ and one by averaging 10,000 samples from the AR decoder, $\pxz$.}
    \label{fig:Sz}
\end{figure}
}

\newcommand\tabsampling{
\begin{table*}[h]
\centering
\caption{
Our denoiser randomly samples clean images for a given noisy image.
A consensus solution can be produced by averaging random samples.
The PSNR of the mean of increasing sample sizes is shown below.
}
\begin{adjustbox}{width=1\textwidth}
\begin{tabular}{l|ccc:ccc:cc}
\multicolumn{1}{l|}{} & \multicolumn{3}{c:}{EMCCD} & \multicolumn{3}{c:}{SCM} & \multicolumn{2}{c}{Simulated} \\
\multicolumn{1}{l|}{No. samples} & Conv. A & Conv. B & Mouse Actin & Mouse Nuclei* & Actin Conf. & Mito Conf.  & FFHQ Stripe  & FFHQ Checkerb. \\ \hline
 1 & 36.54 & 42.33 & 37.43 & 42.25 & 26.81 &  22.62 & 32.27 & 33.03\\
 10 & 37.39 & 43.90 & 39.03 & 42.91 & 27.37 & 23.39 & 35.24 & 35.85  \\
 100 & 37.49 & 44.10 & 39.23 & 42.98 & 27.42 & 27.50 & 35.66 & 36.27 \\
 1000 & 37.50 & 44.10 & 39.24 & 42.99 & 27.44 & 27.52 & 35.74 & 36.32\\
 \end{tabular}
 \end{adjustbox}
 \label{tab:sampling}
 \end{table*}
}

\newcommand\figConvA{
\begin{figure*}[]
    \centering
    \includegraphics[width=0.8\linewidth]{supp_figures/noisy/conva-noisy.pdf}
    
    \vspace{2mm}
    
    \includegraphics[width=0.8\linewidth]{supp_figures/denoised/conva-denoised.pdf}

    \vspace{2mm}
    
    \includegraphics[width=0.8\linewidth]{supp_figures/clean/conva-clean.pdf}
    \caption{\emph{Convallaria A}}
\end{figure*}
}

\newcommand\figConvB{
\begin{figure*}[]
    \centering
    \includegraphics[width=0.8\linewidth]{supp_figures/noisy/convb-noisy.pdf}

    \vspace{2mm}
    
    \includegraphics[width=0.8\linewidth]{supp_figures/denoised/convb-denoised.pdf}

    \vspace{2mm}
    
    \includegraphics[width=0.8\linewidth]{supp_figures/clean/convb-clean.pdf}
    \caption{\emph{Convallaria B}}
\end{figure*}
}

\newcommand\figMouseA{
\begin{figure*}[]
    \centering
    \includegraphics[width=0.8\linewidth]{supp_figures/noisy/mouseactin-noisy.pdf}

    \vspace{2mm}
    
    \includegraphics[width=0.8\linewidth]{supp_figures/denoised/mouseactin-denoised.pdf}

    \vspace{2mm}
    
    \includegraphics[width=0.8\linewidth]{supp_figures/clean/mouseactin-clean.pdf}
    \caption{\emph{Mouse Actin}}
\end{figure*}
}

\newcommand\figMouseN{
\begin{figure*}[]
    \centering
    \includegraphics[width=0.8\linewidth]{supp_figures/noisy/mousen-noisy.pdf}

    \vspace{2mm}
    
    \includegraphics[width=0.8\linewidth]{supp_figures/denoised/mousen-denoised.pdf}

    \vspace{2mm}
    
    \includegraphics[width=0.8\linewidth]{supp_figures/clean/mousen-clean.pdf}
    \caption{\emph{Mouse Nuclei}}
\end{figure*}
}

\newcommand\figActinConfocal{
\begin{figure*}[]
    \centering
    \includegraphics[width=0.8\linewidth]{supp_figures/noisy/actinconfocal-noisy.pdf}

    \vspace{2mm}
    
    \includegraphics[width=0.8\linewidth]{supp_figures/denoised/actinconfocal-denoised.pdf}

    \vspace{2mm}
    
    \includegraphics[width=0.8\linewidth]{supp_figures/clean/actinconfocal-clean.pdf}
    \caption{\emph{Actin Confocal}}
\end{figure*}
}

\newcommand\figMitoConfocal{
\begin{figure*}[]
    \centering
    \includegraphics[width=0.8\linewidth]{supp_figures/noisy/mitoconfocal-noisy.pdf}

    \vspace{2mm}
    
    \includegraphics[width=0.8\linewidth]{supp_figures/denoised/mitoconfocal-denoised.pdf}

    \vspace{2mm}
    
    \includegraphics[width=0.8\linewidth]{supp_figures/clean/mitoconfocal-clean.pdf}
    \caption{\emph{Mito Confocal}}
\end{figure*}
}

\newcommand\figEmbryo{
\begin{figure*}[]
    \centering
    \includegraphics[width=0.8\linewidth]{supp_figures/noisy/embryo-noisy.pdf}

    \vspace{2mm}
    
    \includegraphics[width=0.8\linewidth]{supp_figures/denoised/embryo-denoised.pdf}
    \caption{\emph{Embryo}}
\end{figure*}
}

\newcommand\figStem{
\begin{figure*}[]
    \centering
    \includegraphics[width=0.8\linewidth]{supp_figures/noisy/stem-noisy.pdf}

    \vspace{2mm}
    
    \includegraphics[width=0.8\linewidth]{supp_figures/denoised/stem-denoised.pdf}
    \caption{\emph{STEM}}
\end{figure*}
}

\newcommand\figInfrared{
\begin{figure*}[]
    \centering
    \includegraphics[width=0.8\linewidth]{supp_figures/noisy/infrared-noisy.pdf}

    \vspace{2mm}
    
    \includegraphics[width=0.8\linewidth]{supp_figures/denoised/infrared-denoised.pdf}
    \caption{\emph{IR}}
\end{figure*}
}

\newcommand\figStripe{
\begin{figure*}[]
    \centering
    \includegraphics[width=0.8\linewidth]{supp_figures/noisy/ffhqstripe-noisy.pdf}

    \vspace{2mm}
    
    \includegraphics[width=0.8\linewidth]{supp_figures/denoised/ffhqstripe-denoised.pdf}

    \vspace{2mm}
    
    \includegraphics[width=0.8\linewidth]{supp_figures/clean/ffhqstripe-clean.pdf}
    \caption{\emph{FFHQ - Stripe}}
\end{figure*}
}

\newcommand\figCheckerboard{
\begin{figure*}[]
    \centering
    \includegraphics[width=0.8\linewidth]{supp_figures/noisy/ffhqcheckerboard-noisy.pdf}

    \vspace{2mm}
    
    \includegraphics[width=0.8\linewidth]{supp_figures/denoised/ffhqcheckerboard-denoised.pdf}

    \vspace{2mm}
    
    \includegraphics[width=0.8\linewidth]{supp_figures/clean/ffhqcheckerboard-clean.pdf}
    \caption{\emph{FFHQ - Checkerboard}}
\end{figure*}
}
